# Supplementary material for: Fluent and Low-latency Simultaneous Speech-to-Speech Translation with Self-adaptive Training
Source: arXiv:2010.10048 source file (2020-10-21)
Supplement: Supplementary file 1 [file appendix.tex]

% !TEX root = main.tex
% \begin{itemize}
% 	\item To synthesize fluent target speech, we can only stop synthesizing when reach pause (e.g. comma, period)
% 	\item Before synthesizing pause, don't stop generating new target words from translation model.
% 	\item When synthesizing audio for each target word, encode as many source words as possible.
% 	\item Train TTS model with different pauses, control prosody with pause when decoding.
% \end{itemize}

 \begin{figure*}
 \resizebox{\textwidth}{!}{
 %\centering
 \setlength{\tabcolsep}{1.5pt}
 \begin{tabu}{r | l l l l l l l l l l l l   l l }
 & 1 & 2 & 3 & 4 & 5 & 6 & 7 & 8 & 9 & 10 & 11 & 12 & 13 & 14  \\
   \rowfont{\small}
% & {\textit{N\`ax\={\i}e }}\, & {\textit{z\v{o}ngt\v{o}ng}} & {\textit{z\`ai}}  & \textit{M\`os\={\i}k\=e} & \yu   &\pujing &  \huiwu \\

  & 那些\, & 人 & 热心 & 待 & 你们 & 却 & 不是 & 好意\\
  \rowfont{\small}
  &  those & people & warm-hearted & treat & you & but & not & goodwill &\\
 \hline

 \multirow{2}{*}{wait-$2$} &  & & They & zealously & affect & you & , & but & not & well\\
  &  & & They &  are  & zealous & to & win & you & over & , & but & for & no & good \\
 \hline
 \multirow{2}{*}{SAT-$2$}
  &  & & They & zealously & affect & you & , & but & not & well\\
  &  & & They are  & 
 zealous  to \, & 
 win & 
 you  over \, & 
 ,  but \,  & for & no & good \\
 \hline

% & 1 & 2 & 3 & 4 & 5 & 6 & 7 & 8 & 9 & 10 & 11 & 12 & 13 & 14  \\
  \end{tabu}
 }
 \caption{
 An example in training data.
 \label{fig:idea2}
 }
 \end{figure*}

 \begin{figure*}
 \resizebox{\textwidth}{!}{
 %\centering
 \setlength{\tabcolsep}{1.5pt}
 \begin{tabu}{r | l l l l l l l l l l l l   l l l l l l}
 & 1 & 2 & 3 & 4 & 5 & 6 & 7 & 8 & 9 & 10 & 11 & 12 & 13 & 14 & 15 & 16 & 17 & 18  \\
   \rowfont{\small}
% & {\textit{N\`ax\={\i}e }}\, & {\textit{z\v{o}ngt\v{o}ng}} & {\textit{z\`ai}}  & \textit{M\`os\={\i}k\=e} & \yu   &\pujing &  \huiwu \\

  & 人们\, & 是 & 不合逻辑的 & 、 & 不讲理的 & 并且 & 自我 & 为 & 中心 & 的 & , & 不管 & 怎样 & , & 爱 & 他们\\
  \rowfont{\small}
  &  people & are & illogical &  & unreasonable & and & self & & centered & & & despite & anyway & & love & them &\\
 \hline

 wait-$2$&  & & People &  are  & illogical  & unreasonable & and & self-centered & love & them & anyway\\
 SAT-$2$ &  & & People &  & are &  & illogical &  & unreasonable & & and & & self-centered & & love & & them & anyway\\
 \hline
% & 1 & 2 & 3 & 4 & 5 & 6 & 7 & 8 & 9 & 10 & 11 & 12 & 13 & 14 & 15 & 16 & 17 & 18  \\
  \end{tabu}
 }
 \caption{
 An example in training data.
 \label{fig:idea2}
 }
 \end{figure*}

 \begin{figure*}
 \resizebox{\textwidth}{!}{
 %\centering
 \setlength{\tabcolsep}{1.5pt}
 \begin{tabu}{r | l l l l l l l l l l l l   l l l l l l l l l}
 & 1 & 2 & 3 & 4 & 5 & 6 & 7 & 8 & 9 & 10 & 11 & 12 & 13 & 14 & 15 & 16 & 17 & 18  \\
   \rowfont{\small}
% & {\textit{N\`ax\={\i}e }}\, & {\textit{z\v{o}ngt\v{o}ng}} & {\textit{z\`ai}}  & \textit{M\`os\={\i}k\=e} & \yu   &\pujing &  \huiwu \\

  & 对\, & 牛津 & 来说 & 只 & 出 & 网络版 & 更 & 符合 & 经济效益 \\
  \rowfont{\small}
  &  for & oxford &  & only & publish & online & more & conform & economic benefit\\
 \hline

 wait-$2$ &  & & for & oxford & the & decision & to & go & online & only & would & make & a & great & deal & of & economic & sense \\
 SAT-$2$ &  & & for oxford & the decision & to go & online  only & would make & a great & deal  of & economic & sense \\
 \hline
% & 1 & 2 & 3 & 4 & 5 & 6 & 7 & 8 & 9 & 10 & 11 & 12 & 13 & 14 & 15 & 16 & 17 & 18  \\
  \end{tabu}
 }
 \caption{
 An example in training data.
 \label{fig:idea2}
 }
 \end{figure*}
